# Supplementary material for: Guardian of the HAN: Thwarting Mobile Attacks on Smart-Home Devices Using OS-level Situation Awareness
Source: arXiv:1703.01537 source file (2017-03-07)
Supplement: Supplementary file 1 [file appendixImprovements.tex]

\vspace{3pt}\noindent \textbf{Clarified Motivation}. Concerns were raised that the number of apps without authentication (9/22) is small to motivate the work. However, our app analysis was not designed to be a threat prevalence study since ample evidence already exist. Our goal is to prove that device vendors trust the HAN and mobile adversaries can trivially compromise HAN devices. In previous versions, one section was describing both the motivation and our IoT app study. In this version, “Motivation” discusses existing evidence regarding unguarded smart-home devices and examples motivating the need for proactive defense; “Operations and Existing Trust Model”, describes our study on a small number of smart home apps (55)-but enough for a statistical significance test-which demonstrates IoT vendors’ erroneous trust model. The latter also describes our mobile attacks on such devices.

\vspace{3pt}\noindent\textbf{Broaden Scope.} Concerns were raised that focusing on WiFi smart-home devices is of narrow scope; arguments were based on that (1) a lot of the apps (25/55), still use cloud communications while in the HAN and, (2) since IoT problems are known, the vendors probably fixed them. To address (1), we (a)  enhance this version with new industry examples illustrating  an increasing support for local computations (e.g. Smartthings now runs smart apps locally), (b) broaden the scope: we explain how Hanguard can also tackle remote adversaries (Security Analysis:Beyond the app-level adversary) and how its RBAC access control can extend to cloud-based apps (Discussion:Communication through cloud). Regarding (2), we argue that device vulnerabilities are a long standing issue and a proactive, device-independent approach is a step towards the right direction.

\vspace{3pt}\noindent\textbf{Simplified Threat Model.} Our adversary model was indeed confusing. In this version we clearly focus on the mobile-app adversary. Defense against other adversaries is discussed in a different section (“Security Analysis:Beyond the app-level adversary”).

\vspace{3pt}\noindent\textbf{Performed Security Analysis.} Some of our reviewers requested a security analysis while others tried to point out security flaws. We added text when appropriate to clarify Hanguard’s design. More importantly, we performed a security analysis, presented in a new Section(“Security Analysis”).

\vspace{3pt}\noindent\textbf{Clarified Policy Generation.} We discuss in text how Hanguard creates default rules to ease user burden. Moreover, we clarify that Hanguard does not expect users to write policy rules but to just match users, apps and devices.

\vspace{3pt}\noindent\textbf{Performance on iOS.} Concerns were raised that our system is impractical for iOS (app  latency and throughput). However, only policy-protected apps on iOS, performing real time streaming, are affected in practice; most IoT apps send and receive simple commands/messages. Our thorough evaluation shows that. We clarify in text the challenging cases where performance is hindered in practice.

\vspace{3pt}\noindent\textbf{Other Additions.} We utilized the appendix space to provide a complete functionality categorization stemming from 353 manually inspected IoT products. We have further added details on the 55 IoT apps selected for our statistical significance test, including Android package names and our analysis results. We believe our data will be useful to other researchers studying IoT security.
