# Supplementary material for: Guardian of the HAN: Thwarting Mobile Attacks on Smart-Home Devices Using OS-level Situation Awareness
Source: arXiv:1703.01537 source file (2017-03-07)
Supplement: Supplementary file 3 [file appendixPastReviews.tex]

%appendixPastReviews
\subsection{ISOC Network and Distributed System Security Symposium 2017 (NDSS '17)}
\subsubsection{NDSS '17 Review \#237A}

\begin{itemize}
\item Overall merit: 2. Weak reject
\item Reviewer expertise: 3. Knowledgeable
\end{itemize}
%\vspace{3pt}\noindent\textbf{Overall merit:} 2. Weak reject
%\vspace{3pt}\noindent\textbf{Reviewer expertise:} 3. Knowledgeable



\vspace{3pt}\noindent\textbf{Paper summary.} The paper addresses the problem of using a Home Area Network as a trusted network for IoT devices. The proposed design includes modification to the router and a user-space Monitor app for each mobile device. The Monitor app uses side-channel and the ability to proxy network traffic to collect the context of the mobile device and forwards it to the router. With such OS-level context information, the router is able to enforce security policies and route traffic accordingly.

\vspace{3pt}\noindent\textbf{Paper Strengths.}


+ Fairly well written and easy to understand.


+ Works across both iOS and Android -- the two major mobile platforms.


+ Does not require changes to IoT devices.


+ Well-defined adversary model. Clear discussion of adversary capabilities and how to counter them.


\vspace{3pt}\noindent\textbf{Paper weaknesses.}

- Motivation is not sufficiently compelling.


- Non-trivial performance overhead on iOS devices.


- Deployment is complex. Requires changes to the router and app on mobile devices. Each IOT device also needs to be registered with the security policy.


- Significant threats outside the assumed adversary model.


\vspace{3pt}\noindent\textbf{Additional comments for author.} The paper is overall well written. It lays down the problem statement clearly and discusses the solution in great detail. However, I feel that the motivation could be more compelling. In particular, the authors examined 92 IOT devices with mobile applications, but found only 21 of them with local wifi connections and only 8 with an unauthenticated connection. Moreover, only 4 of them are described in detail in the paper, 3 of them from the same manufacturer and the 4th one with less than 500 downloads on app store. The prevalence of cloud-connected IOT devices with authentication suggests that the problem may not be a critical one. 


The design description is clear and comprehensive. It covers both iOS and Android devices. However, for iOS devices, excessive performance overheads are reported. 100ms RTT and 30% throughput is rather unacceptable for real-world deployment. 


Although the system does not require modifications to the IOT devices, it does require changes to the router. In addition, each new IOT device (as well as each new phone) needs to be registered with the security policy. Although this would not hurt the operation or feasibility of the system, it does affect usability and scalability.


While the adversary model is well defined and clearly discussed, there are significant challenges that arise from the system design. For example, the system relies on IP address to identify the device and the package name (uid) to identify the app. A new device can easily use ARP spoofing to bypass the guest device role policy. And similarly, a malicious app can install itself with the same package-name as the official app and access its permissions. There are several traditional threats outside the assumed threat model that make the system's attack-resiliency questionable.

\subsubsection{NDSS '17 Review \#237B}

\begin{itemize}
\item Overall merit: 2. Weak reject
\item Reviewer expertise: 4. Expert
\end{itemize}
             	


\vspace{3pt}\noindent\textbf{Paper summary.} The paper proposes Hanguard, a system that protects WIFI-connected IoT devices from malicious apps on mobile devices connected to the same HAN (home area network). Hanguard consists of a non-privileged app on a mobile device and a customized router. The app monitors access from the mobile device to IoT devices and controls the router to allow/deny such accesses. Hanguard mitigates unauthorized access from mobile to IoT devices whose authentication is given to the entire HAN or mobile devices, as opposed to individual apps.


\vspace{3pt}\noindent\textbf{Paper Strengths.}


+ The paper addresses a real and interesting problem (though the scope of the proposed solution is somewhat limited, more on this later)


+ Hanguard doesn't require any changes to IoT or mobile OS, which will ease adoption and deployment in practice. The authors demonstrated Hanguard on both Android and iOS devices. 


+ The system design is straightforward and the evaluation is thorough.


\vspace{3pt}\noindent\textbf{Paper weaknesses.}


- The work is motivated by a bigger problem than it actually solves, which is probably fine as the first step toward full solutions. Hanguard only considers IoT connected via WIFI/LAN while leaving out devices connected/controlled via Bluetooth, NFC, etc., some of which were shown to be vulnerable to the same attack. 


- The addressed problem is not really as new as the paper claims. There were many studies, from both the industry and academia, that revealed the weak authentication used by IoT devices, especially the early generations. Thanks to those studies, many IoT vendors have already adopted simple and effective countermeasures. Therefore, I suspect that there might not be that many IoT devices that are still vulnerable. The fact that the paper only found 4 vulnerable devices (3 from the same vendor) makes me feel the problem is mostly solved in reality. 


- Although I appreciate the system building efforts went into this work, the novelty of the work seems quite limited. The so-called "situation awareness" is just network traffic proxy/sniffing. 


- Generating policies for Hanguard requires lots of assistance by end users, who may not be capable of understanding or correctly configuring the system. Some discussion on if policy generation can be made easy or automatic will help ease concerns about how useful Hanguard could be to average users. On the other hand, the current policy model seems a bit narrow. For instance, it's unclear if it can support apps that are supposed to control multiple IoT devices.


\vspace{3pt}\noindent\textbf{Additional comments for author.} Some related works are missing, such as those that discussed similar attacks on Bluetooth devices, e.g., “Inside job: Understanding and mitigating the threat of external device mis-binding on android”

\subsection{ACM Conference on Computer and Communications Security 2016 (CCS '16)}
\subsubsection{CCS '16 Review \#112A}

\begin{itemize}
\item Overall merit: 3. Weak reject - will not argue against
\end{itemize}  

\vspace{3pt}\noindent\textbf{Paper summary.} The paper deals with an important issue of enabling security in Home Area Networks (HANs) in which IoT devices trust all other devices connected to the same network. Authors propose a system that enforces access control policies to block malicious applications from accessing IoT devices. They implemented a Monitor app that runs on a mobile phone and identifies whether any application tries connecting to a protected IoT device. It informs the router through a secure channel whether the access can be granted. The router runs modified version of firmware that enforces the decisions.


The authors crawled 353 apps for controlling IoT devices and manually analysed their security protections. More than a half misses correct mechanisms. However, only 11 out of 20 apps fits to the vector attack discussed by this paper which implies rather limited scope of this work. Authors claim that this is because the problem is relatively new and claim that local connectivity within a HAN network without necessity of using Internet or Bluetooth is a new trend.


\vspace{3pt}\noindent\textbf{Paper strengths.} The paper provides insight into implementation of both phone and router side software. The solution uses role based access control to protect devices. It discusses two different implementations for iOS and Android. The first one uses VPN for protected applications to identify connections to the IoT devices. The second uses side channels to analyse current phone’s kernel data structures.


The authors conduct exhaustive evaluation and provide links to videos in which they demonstrate their solution. Using 4 IoT devices they confirm the effectiveness of the system.  They analyse the performance of the system and impact on the resource consumption, battery lifetime, and decision latency. They also discuss the communication overhead and application throughput. The impact of the proposed system is minimal on the performance of the mobile phone and the router.
Connections to prior work in the field are made. The work is well set in context and contrary to other solutions it also analyses the cases when the original mobile device is also compromised (attacks from a trusted phone, but not a trusted app).
The paper is well written and easy to understand.


\vspace{3pt}\noindent\textbf{Paper weaknesses.} The paper is very applied and I miss some long-term contribution.


\vspace{3pt}\noindent\textbf{Response to rebuttal.} Thank you for your additional explanations on the long-term contribution. I now understand your point on system architecture using phones as monitors for local area SDN.


\subsubsection{CCS '16 Review \#112B}
\begin{itemize}
\item Overall merit: 2. Reject - will argue against
\end{itemize}




\vspace{3pt}\noindent\textbf{Paper summary.} This paper examines the challenge of securing Internet of Things devices connected to Home Area Networks, which are often controlled through mobile apps over Wifi connections. For those apps where Wifi is the primary communication conduit, a central point in the home environment would be the router, so the argument in this paper is that the router is where enforcement of protections against possibly malicious mobile apps can be placed. The solution in this paper, Hanguard, is a system devised to work on mobile devices as well as on routers, designed in an SDN-like fashion. A controller runs on the router. A Monitor app runs on mobile devices while the router would be patched to support kernel level extensions to perform enforcement. Policy is specified and enforced in an RBAC-like fashion with a type enforcement system strongly inspired by SELinux. Solutions are developed for Android and iOS and for a router running OpenWRT. An evaluation considers the effectiveness of the approach and benchmarks based on computation, power, and bandwidth.


\vspace{3pt}\noindent\textbf{Paper strengths.}


- novel idea in terms of not relying on a converged system like HomeKit or Smart Things to provide protection but rather focusing on the commodity environment


- fully implemented for both iOS and Android, as well as creating a real OS patch for a WRT router to be able to use.


\vspace{3pt}\noindent\textbf{Paper weaknesses.}


- Unclear who writes or administers policy for something that looks a lot like SELinux; far too complex for end-users


- Unclear what the semantics of using type enforcement in conjunction with the seemingly orthogonal Category tag actually are


- Not clear whether mobile malware is actually a real problem


\vspace{3pt}\noindent\textbf{Additional comments for authors.} This was an interesting new take on the IoT protection problem. I was particularly impressed that you implemented an end to end solution incorporating both Android and iOS as well as an actual router OS, and a detailed description of how the monitors work on all of these architectures.


I have a lot of questions about Section 2. The authors boldly claim that fixing security issues in IoT devices for the home is difficult, but depending on the device in question, these can have a substantial amount of computational power to be able to perform upgrades. It seems like a terrible idea for manufacturers to make Internet-addressable devices that can't be upgraded and I don't know if I believe that this is the reality; at the very least you should cite sources that attest to the inability of these devices to be fixed. On a side note, there are a lot of citations in this paper, and while I appreciate comprehensive research, a lot of these are variants of IoT devices. Many could be safely removed without affecting the narrative, leaving more space for discussion of other points relevant to the paper. 


You write that you cannot buy a lot of devices, but what about analyzing firmware updates? That might tell you more than examining mobile apps, which are merely communicating with the IoT device but not providing the control mechanisms. The manual analysis was a little surprising to me. Manually examining 223 IoT apps is a lot of work, but there was no complete methodology of how you determined the functionality you were looking for. Did you consider running Mallodroid [A] to determine potential weaknesses in the apps? You might want to look at Reaves et al.'s work on mobile money app analysis [B] to see an example of a methodology for manual analysis. I'm also not sure why you removed all apps that had Bluetooth permission - were these Bluetooth-only? The authors write about a "milder effect" on false negatives, and I don't really know what that means.


For that matter,  while it seems problematic that these IoT devices have no authentication, it's less clear that the problem is mobile malware. In Section 3.1 the authors write "We have already seen the explosion of mobile malware in the wild", which comes as a surprise given work showing that mobile malware is not really much of a problem at all [C]. Please cite your justification here. I would postulate that routers are in fact the more likely place where an infection would happen, since how often do users update their routers compared to their mobile phones?


I'm not sure who is supposed to be in charge of labeling the IoT devices. Probably not the devices themselves, and do the apps know enough to be able to set types and other label attributes? Is this up to the router? Or the user setting up the enforcement architecture? If so, it's worth noting that experienced administrators struggle with SELinux policies, so this would be virtually hopeless in the home environment if the user needs to ever debug these policies. It's also unclear what the semantics of the category tag are; is policy monotonic if category is a choice? Some formal understanding of the semantics of this scheme would be helpful. Also is the idea that if mandatory access control mechanisms are in place that there are reference monitor guarantees provided by the controller? If so, how are they verified?


In Section 4.2, it is unclear how the comparison between NAÏVE and SMARTER modes compares with the "popular and mature apps" considered in Figure 12. You're comparing an actively scanning A/V app (which NAÏVE/aka SIMPLE comes quite close to in terms of energy consumption) to an app that is on all the time (presumably the A/V software is not scanning all the time). Also what type of activity is happening on GMAIL? Is it actively pulling down data or is this "idle" mode of just periodically checking for new mail? It's hard to know how fair this comparison actually is. The TCP Monitor on iOS shows that there is probably going to be a significant energy impact given the CPU utilization, which is almost as high as the A/V program in scanning model.


Finally, there was recently a paper on analyzing smart home applications [D] that is highly related; the authors should look at and cite this work.


[A]  S. Fahl, M. Harbach, T. Muders, L. Baumgärtner, B. Freisleben, M. Smith, Why Eve and Mallory Love Android: An Analysis of Android SSL (in)Security, in: Proceedings of the 2012 ACM Conference on Computer and Communications Security, ACM, New York, NY, USA, 2012: pp. 50–61.


[B] B. Reaves, N. Scaife, A. Bates, P. Traynor, K.R.B. Butler, Mo (bile) Money, Mo (bile) Problems: Analysis of Branchless Banking Applications in the Developing World, in: 24th USENIX Security Symposium (Security’15), Washington, DC, USA, 2015. 


[C] C. Lever, M. Antonakakis, B. Reaves, P. Traynor, W. Lee, The Core of the Matter: Analyzing Malicious Traffic in Cellular Carriers, in: NDSS, 2013.


[D] E. Fernandes, J. Jung, A. Prakash, Security Analysis of Emerging Smart Home Applications, in: IEEE Symposium on Security and Privacy, 2016. doi:10.1109/SP.2016.44.


\vspace{3pt}\noindent\textbf{Response to rebuttal.} Thanks for taking the time to write the rebuttal. I appreciate that you will consider the feedback, though it doesn't sway my overall opinion of the work right now.


\subsubsection{CCS '16 Review \#112C}
\begin{itemize}
\item Overall merit: 3. Weak reject - will not argue against
\end{itemize}
                  	

\vspace{3pt}\noindent\textbf{Paper summary.} This paper aims to protect smart-home IoT devices from unauthorized access by non-root malware on legitimate client devices or unauthenticated devices in the same HAN (Home Area Network). The authors first conduct an extensive investigation on the current status of IoT smart-home devices available on the market, and identify a handful of vulnerable devices that lack proper authentication. Assuming that IoT manufacturers won't be able to fix these issues quickly. An SDN-like approach is proposed to solve this class of problem. The solution requires changing the router software which will work together with a monitor app deployed on smartphones. The router can block communication attempts initiated by unauthorized apps and allow the authorized ones (attested via a control message sent by the monitor app). Through evaluation on a real system implemented on both the client and the router, it is shown to protect this class of threats without significant overhead.


\vspace{3pt}\noindent\textbf{Paper strengths.}


It is an interesting approach to solve an important problem.


The proposed solution appears to be secure as it is relatively straightforward to reason.


Nice measurement result in the beginning.


Significant effort is put into implementation and evaluation. It is believable that the system can work in practice.


\vspace{3pt}\noindent\textbf{Paper weaknesses.}


The motivation is a little weak. Only 20 out of 223 IoT systems support local communication. The authors claim that this is becoming the trend (since they are released in mid-2014) but it is unclear when the remaining IoT systems are released and why they do not support local communication.


There are several design decisions and evaluation results that are puzzling to me (more details later). 


The deployment cost seems still relatively high. The initial setup phase involves many steps: flashing the router firmware, installing an app on the smartphone, configure the SSL/TLS for the connection between the app and the router, establishing the username and password for the monitor-to-router communication, and configure the policy for each IoT device at home.


The fact that the solution on Android relies on frequently polling side channels worries me. This represents the first-of-its-kind legitimate use of side channels, which makes the detection of malware utilizing side channels more difficult. It is also unclear whether such information will be made available in the long run.


\vspace{3pt}\noindent\textbf{Additional comments for authors.} The authors argue that IoT devices are hard to patch, but there is not enough supporting evidence. Are there any concrete examples where patches are not released even when serious flaws of IoT devices are discovered?


Why do we need distributed policy update when the router alone can keep the latest policy? The smartphones shouldn't need to store the policy. They just need to query the router and perhaps cache the current policy. In addition, the master phone should be allowed to update the policy stored on the router. This avoids all the complicated distributed synchronization that is introduced.


Allowing client-side to do the app-level check is risky if the client itself is malicious. Why not just send the host information to router and let router do both app-level and phone-level checks. 


There appears to be a security flaw in the current system. Currently, the cached entries in PFDC are not purged quickly enough on the router (it seems to be purged only when it runs out of space). The entries technically should be removed as soon as the client closes the connection (e.g., TCP FIN or TCP RESET). This requires the router to become a stateful firewall that accurately manages the lifecycle of TCP connections (which may not be easy). In addition, in the UDP case, it is difficult to determine when the connection is closed. If not dealt with properly, the malware can reuse the port number of a previously legitimate connection and gain unauthorized access.


The overhead is quite significant. Polling every 5ms obviously is going to hurt battery as the authors show. Specifically, even the SMARTER mode consumes comparable power to gmail. However, we have to keep in mind that the solution is incurring ADDITIONAL power on top of whatever foreground apps are incurring. So if a user is running gmail, now the power consumption almost doubles. This is clearly undesirable. 


I don't understand the result shown in Figure 13. Even considering the most aggressive 10ms polling interval, the average delay to catch a new TCP connection is going to be 5ms. And 5ms is a LONG TIME in the computer world (millions of instructions can be executed), the OS must have been able to push out the original TCP SYN packet well before your program can push out anything. How is it possible that your control packet can arrive ahead of time most of the time (as shown in Figure 13)? This simply does not make any sense.


\vspace{3pt}\noindent\textbf{Response to rebuttal.} Thanks for the rebuttal. It clarified some things. But I'm still a bit puzzled by the design decision of keeping state on the phones instead of on the router. It complicates things even more when you add PDFC on the router (which is actually a copy of the state on the phone). Managing the same state at two places can inherently be challenging and error-prone. The authors may want to explain this more in the future version.



\subsubsection{CCS Rebuttal}

Thanks for your constructive feedback.


\#112A
[Long-term contribution]. We believe our system architecture using phones as monitors for local area SDN is promising and might be applicable to different domains.


\#112B
[Who writes policies]. We do *NOT* expect the users to write SELinux policies. The user only needs to map a small set of users, IoT devices and installed apps, if default associations need modification. The way SELinux-compatible policies are created is transparent to the user.


[Type-enforce/category-tag]. *Multi-category security (MCS) is not our construct; it’s an SELinux construct*. This is also used on Android to enforce the multi-user functionality. As with SELinux and SEAndroid, the MCS check is applied after the type enforcement so it can only further restrict security. 


[Mobile-malware not real problem]. Reports show low infection rates in the US but are highly variable [2] depending on the datasets/methodologies. Also increasingly there are potentially-harmful-apps, particularly in places like China.  The mere presence of mobile malware given the ease of distribution (e.g. self-signed apps, third-party app markets) and the rise of mobile malware [3,4,5], render it a security threat. Mobile malware is the focus of many respected academic works [6,P103,P66,P101] and a public concern [7,8,9].


The Bluetooth filter eliminated some interesting to us apps but allowed us to quickly remove almost all of the apps for wearables. 


[IoT upgrades].  We do not assume lack of software upgrades on *ALL* devices. Most challenging are hardware upgrades (see the Square dongle case [1]). 


[You write that you cannot buy...]. We appreciate the references. We'll provide more details on our app analysis. Our goal was to find even more evidence of security issues on IoT devices. Towards this, our approach has multiple benefits: (1) we can easily acquire apps; (2) there is no cost; (3) it’s generally easier/faster to analyze Android apps than firmware. 


\#112C
[Deployment cost]. Please note that commodity routers already offer apps; the user just needs to approve the firmware update through their app; SSL/TLS is established transparently to the user; default policies are automatically created.


[Relying on polling]. Side-channels were used for defense before [P100]; please note that Hanguard can be implemented without them (Section 5).


[Design: client-side]. Since we trust the information received from the Monitors, we can trust them with the app-level check. Performing computation/storage at the data source is a performance decision.


[Alleged flaw]. Monitors are *INVALIDATING* flows: all app-level decisions are made by Monitors; the router simply enforces them and doesn’t need to remember any states. PFDC-entry-purging is a measure against DoS. 


General Concerns
[Motivation]. Please note that Hanguard does not only protect vulnerable devices but its RBAC enables authorization management for all devices. Edge computing is a driving force for local computation.


[1] http://goo.gl/G0Vji7

[2] Faruki,Parvez,et al."Android security: a survey of issues, malware penetration, and defenses."IEEE Communications Surveys\&Tutorials.

[3] https://goo.gl/lhZ1yb

[4] http://goo.gl/3f1LP8

[5] http://goo.gl/VfUKB4

[6] Arp,Daniel,et al."DREBIN: Effective and Explainable Detection of Android Malware in Your Pocket."NDSS.2014.

[6] http://goo.gl/4YbaWg

[7] http://goo.gl/RE5ffK

[8] http://goo.gl/EUGmDC


[Px] Citation in the paper~\footnote{the version that was submitted at CCS '16} with number x.

\subsection{USENIX Security Symposium 2016 (Security '16)}

\subsubsection{Security '16 Review \#187A}
\begin{itemize}
\item Overall merit: 2. Weak paper. This paper should be rejected but I will not fight strongly against it.
\item Reviewer expertise: 3. Knowledgeable
\end{itemize}

\vspace{3pt}\noindent\textbf{Paper summary.} This paper identifies a lack of authentication between IoT vendor phone apps and
devices as an emerging problem, and proposes Hanguard as an approach for
retrofitting such authentication onto otherwise secure IoT devices.


\vspace{3pt}\noindent\textbf{Paper Strengths.}


+ IoT security is a relevant problem area


\vspace{3pt}\noindent\textbf{Paper Weaknesses.}

- Confusing threat model

- Approach relies on unrealistic or fragile assumptions


\vspace{3pt}\noindent\textbf{Comments for author.} Perhaps unsurprisingly, some IoT vendors are giving short shrift to security,
and so we have IoT devices that can be controlled by unauthenticated apps that
can access the local WiFi network.  Hanguard makes some good, practical
assumptions; for instance, assuming that vendors will be slow to fix these
problems, and therefore Hanguard avoids modifications to IoT devices or vendor
apps themselves in favor of a separate monitor app on the phone and changes to
the wireless router.


However, I'm not sure I buy other assumptions that are made by Hanguard.  First
of all, Hanguard is pitched as being able to deal with three separate adversary
models: remote adversaries, fully compromised phones, and malicious phone apps.
"Fully compromised" however is quite strong – e.g., equivalent, I assume, to a
system-level app with root privileges on Android.  In such a scenario, what
prevents malware from extracting whatever secrets it needs from the monitor app,
killing the monitor, and then spoofing control messages?  I would like to see an
explicit argument as to why such an attack isn't actually possible.


The other major problems with this approach are the unrealistic or fragile
assumptions made with respect to the information gathering approaches on Android
and iOS.  First, the iOS approach requires an MDM server to selectively route
per-app traffic through the VPN, which in my opinion is simply a non-starter.
As a matter of necessity, this requires the IoT vendor to push policies through
MDM, and if you're going to require that, wouldn't it be simpler to just add
authentication between devices and apps?


On the other hand, the Android monitor relies on side channels exposed by
`/proc`.  This is widely regarded as a misfeature, and therefore fragile as one
would assume this channel will be closed at some point.


The paper also has some language issues scattered throughout.


- p.1: "to the attack from malicious apps" $\rightarrow$ "to attacks from malicious apps"

- p.1: "6.4 billion of IoT devices" $\rightarrow$ "6.4 billion IoT devices"

- p.11: "mice flows"?

- p.13: "conciously" $\rightarrow$ "consciously"


\subsubsection{Security '16 Review \#187B}
\begin{itemize}
\item Overall merit: 2. Weak paper. This paper should be rejected but I will not fight strongly against it.
\item Reviewer expertise: 3. Knowledgeable
\end{itemize}

\vspace{3pt}\noindent\textbf{Paper summary.} The paper proposes a solution to restrict the control of IoT devices
managed through smartphones connect to local wireless routers. The main
idea is to partition the local network and have an app running on the
phone to gain more knowledge of the network activity and connectivity
to the wireless router.

\vspace{3pt}\noindent\textbf{Paper Strengths.}


Problem is important, IoT attacks have been shown recently and their
number is likely to increase.


They conduct some analysis on a number of apps available in several apps markets.


Includes some interesting technical details.


\vspace{3pt}\noindent\textbf{Paper Weaknesses.}


Attacker model not specified.


Contribution is limited and difficult to evaluate without a clean attacker model.
Seems to push the trust on the monitoring app.


\vspace{3pt}\noindent\textbf{Comments for author.} The paper proposes an interesting solution that deals with an important
problem with no manufacturer solution is sight. The proposed solution has
its own limitations. One of the aspects that makes it difficult to evaluate
the effectiveness of the solution is the lack of a clear definition of the
attacker model. For example, it will be useful if the paper included a picture
showing the current setup, who communicates with whom, under what credentials,
what is provided by the phone already, etc. Is the attacker a compromised app?
Is the attacker a compromised phone? Is the model where somebody else brings 
a compromised phone in a HAN, or a currently used phone is compromised and what
exactly is the attacker assumed to control. The solution requires for some secure
setup to take place between the phone and router, does it assume that any attack
or compromise takes places afterwards?


The solution is quite straightforwards and ultimately consists on an app monitoring
the the Proc files looking for tcp and udp activity. Two questions arise: one relates
to the novelty -- aren't some of the intrusion detection schemes already doing that
and the idea is just adapted for Android; the second -- who is the attacker and where
is the trust pushed with the proposed solution. One for example might say that the
new attacker's goal would be to compromise the monitoring app. 


Some security analysis is needed, the evaluation basically consists of showing that
one particular attack scenario possible before HanGuard (the framework designed in 
this work) is deployed, is now no longer possible.


Overall, while the problem is important and there are some interesting technical
aspects in the paper, overall the solution is not convincing .
